# Supplementary material for: Multi-resonant high-Q plasmonic metasurfaces
Source: arXiv:1907.00458 source file (2019-08-16)
Supplement: Supplementary file 1 [file Multiresonant_SLR_SI.pdf]

# Supporting Information: Multi-resonant high-$Q$ plasmonic metasurfaces

Orad Reshef[1,*], Md Saad-Bin-Alam[2], Mikko J. Huttunen[3], Graham Carlow[4], Brian T. Sullivan[4], Jean-Michel Ménard[1], Ksenia Dolgaleva[1,2], and Robert W. Boyd[1,2,5]

[1] *Department of Physics, University of Ottawa, 25 Templeton Street, Ottawa, ON K1N 6N5, Canada*

[2] *School of Electrical Engineering and Computer Science, University of Ottawa, Ottawa, ON K1N 6N5, Canada*

[3] *Photonics Laboratory, Physics Unit, Tampere University, P.O. Box 692, FI-33014 Tampere, Finland*

[4] *Iridian Spectral Technologies Inc., 2700 Swansea Crescent, Ottawa, ON K1G 6R8, Canada*

[5] *Institute of Optics and Department of Physics and Astronomy, University of Rochester, Rochester, NY 14627, USA*

[*] *Corresponding author: orad@reshef.ca*

The attached code was used to generate the lattice sum figures in the attached manuscript. Up-to-date LSA FP code is provided for free at doi:10.5281/zenodo.3259084. Users of this code are kindly requested to acknowledge and cite its original description and use in this work.

---

```
function LSA_FP
% After setting the inputs (Input), calculates the lattice sums for a periodic
% array consisting of Lorentzian scatterers (plasmonic nanoparticles). In
% addition, the code also considers an additional coupling mechanism
% between the particles via reflection of the scattered field at the
% superstrate-air interface:

% By Mikko J. Huttunen and Orad Reshef
% Last edited, 28.6.2019
%
% Code to calculate transmission spectra of nanoparticle lattices, where an
% additional coupling mechanism is included due to reflection from a top interface.
%
% The code can be used to either
%  1) Calculate a single transmission spectrum
%  2) Sweep over the cladding thickness (Tc) to make 2D transmission spectra
%
% Calculations are based on the lattice sum approach. Please find the
% details from the related papers. Users of this code are kindly requested
% to acknowledge and cite its original description and use in this work.
%
%  1. Huttunen M. J., Dolgaleva K., T?rm? P. & Boyd R. W. Ultra-strong
%  polarization dependence of surface lattice resonances with out-of-plane
%  plasmon oscillations. Opt. Express 24, 28279?28289 (2016).
%
%  2. Reshef O.,  Saad-Bin-Alam Md., Huttunen M. J., Carlow G., Sullivan B. T.
%  Menard J.M., Dolgaleva K., Boyd R. W. Multi-resonant high-Q plasmonic
%  metasurfaces. Under review (2019).
%
%%

%%%%%%%%%%%%%%%%%%%%%%%%%%%%%%%%%%%%%%%%%%%%%%%%%%%%%%%%%%%%%%%%%%%%%%%%%%
%                                                                        %
%  USER INPUT                                                            %
%                                                                        %
%%%%%%%%%%%%%%%%%%%%%%%%%%%%%%%%%%%%%%%%%%%%%%%%%%%%%%%%%%%%%%%%%%%%%%%%%%

%% 1. Lattice, particle and simulation parameters
Input.lambda_peak=1085*1e-9;                      % LSPR center wavelength // 1085 nm
Input.p=[500 1060]*1e-9;                          % Lattice periodicity // 500 nm x 1060 nm
Input.Njj=[400 ; 900]; %  [Nx ; Ny ]              % Array sizes // 400 particles x 900↙
particles
TC=[0.0:0.025:5]*1e-6;                            % Cladding thickness // 0...6 microns↙
0.0:0.025:5
                                                  % may be a single value
                                                  % or a vector range
% wavelength scan range
Input.lambda_min = 800e-9;                        % Min wavelength // 600 nm
Input.lambda_max = 1600e-9;                       % Max wavelength // 1600 nm
lambda_inc = 2.5e-9;                              % Wavelength increments // 2.5 nm
Input.range.wl=Input.lambda_min:lambda_inc:Input.lambda_max;

% Dispersive refractive index for SiO2 cladding (Malitson & Sellmeyer):
wl_mu=Input.range.wl*1e6; % lambda in microns
n_squared=1+0.6961663.*wl_mu.^2./(wl_mu.^2-0.0684043^2)+...
       0.4079426.*wl_mu.^2./(wl_mu.^2-0.1162414^2)+...
       0.8974794.*wl_mu.^2./(wl_mu.^2-9.896161^2);
Input.n_disp=sqrt(n_squared).';

% Optionally, uncomment if you would like dispersionless cladding:
% Input.n=1.445;              % refractive index
% Input.n_disp=Input.n;
```

```
%%%%%%%%%%%%%%%%%%%%%%%%%%%%%%%%%%%%%%%%%%%%%%%%%%%%%%%%%%%%%%%%%%%%%%%%%
%                                                                       %
%  END OF USER INPUT                                                    %
%                                                                       %
%%%%%%%%%%%%%%%%%%%%%%%%%%%%%%%%%%%%%%%%%%%%%%%%%%%%%%%%%%%%%%%%%%%%%%%%%

conversion_factor=1239.84187e-9;   % conversion factor for wl in nm to output in eVs
Input.range.eV=conversion_factor./Input.range.wl;

%% 2. Calculation of the sweep
tic
calc_count=1;
Tot_calcs=length(TC);
Transmission2D = zeros(length(TC), length(Input.range.wl));
for ii=1:length(TC)
    [~,Result(ii)] = Calculate_dipole_sum_Mres_fit_sub(TC(ii),Input);
    calc_count=calc_count+1;

    Transmission2D(ii,:)=Result(ii).T;

    toc_end=toc;
    if ~mod(ii,10) % only show every 10th calculation status
        disp(['Calculating ' num2str(calc_count-1) '/' num2str(Tot_calcs) ...
              ', '  num2str(round(toc_end/ii*(length(TC)-ii))) ' sec remaining.'])
    end
end

%% 3. save calcs:
Save_calculations()

%% 4. Plot results:
close all
if length(TC)>1
    % 2D transmission plots
    fig = figure;
    set(fig,'defaultAxesFontSize',18) % Makes font bigger

    surf(rot90(Input.range.wl,2)*1e9, TC*1e6, squeeze(Transmission2D))
    view(2)
    shading flat
    axis tight
    caxis([0 1])
    ylabel('cladding thickness (\mu{}m)')

    %flipped hot colormap
    hot_inv=colormap(flipud(hot));
    colormap(hot_inv)
    c = colorbar;
    c.Label.String = 'transmittance';
    caxis([0 1])
else
    % 1D transmission plots
    fig = figure;
    set(fig,'DefaultLineLineWidth', 2, 'defaultAxesFontSize',18) % Makes lines thick,↙
font bigger

    plot(rot90(Input.range.wl,2)*1e9, squeeze(Transmission2D), 'k')
    ylabel('transmittance')

    xlim([Input.lambda_min Input.lambda_max]*1e9)
    ylim([0 1.1])
end
xlabel('wavelength (nm)')
```

```
pbaspect([360 270 1])

disp(['Complete in ' num2str(toc) ' seconds.'])

%% (nested) sub-function for making the filename and saving the calculations.
    function Save_calculations()
        % make filename and save calcs.
        if length(TC) == 1
            savename=['Result_Nx' num2str(Input.Njj(1)) '_Ny' num2str(Input.Njj(2)) ...
                '_px' num2str(Input.p(1)*1e9) ...
                '_py' num2str(Input.p(2)*1e9) '_TC' num2str(TC(1)*1e9) ...
                '_LSPR' num2str(Input.lambda_peak*1e9)];
        else
            savename=['Result_Nx' num2str(Input.Njj(1)) '_Ny' num2str(Input.Njj(2)) ...
                '_px' num2str(Input.p(1)*1e9) ... %'_N' num2str(Input.Njj(1))
                '_py' num2str(Input.p(2)*1e9) '_TC' num2str(TC(1)*1e9) '_' num2str(TC↙
(end)*1e9) ...
                '_LSPR' num2str(Input.lambda_peak*1e9)];
        end
        save(savename)
        disp(['Saving file: ' savename])
    end
end


function [Lattice,Result] = Calculate_dipole_sum_Mres_fit_sub(Tc,Input)
% Calculates the lattice sums, contructs polarizability and the Result structure
% containing the data.

Input.plotting=false;                              % handle to control plotting of↙
lattice sums, and polarizabilities
wl_to_eV=1239.84187e-9;                            % conversion coefficient E (eV) =↙
1240nm/lambda(nm)
c=2.9979e8;                                        % speed of light in vacuum

lambda=rot90(rot90(wl_to_eV./Input.range.eV(:)));  % wavelength (m)
k=2*Input.n_disp.*pi./lambda;                      % amplitude of the wavevector

% enforce Njj to be even number, odd numbers break the method
for jj=1:length(Input.Njj)
    if mod(Input.Njj(jj),2)
        Input.Njj(jj)=Input.Njj(jj)+1;
    end
end

%% 1. Calculate lattice sums:
[Lattice,~] = Calculate_lattice_sum_FP_sub(Input,k,Tc);
% S_n_sum=(Lattice.S).';                      % Lattice sum neglecting the interface effect
S_n_sum=(Lattice.S+Lattice.S_FP).';      % Lattice sum including the interface (F-P)↙
effect

% rolling averaging to smooth the lattice sum
windowSize = 6;
b = (1/windowSize)*ones(1,windowSize);
S_n_sum = filter(b,1,S_n_sum);

%% 2. Construct polarizability
lambda_peak=Input.lambda_peak;           % LSPR center wavelength
Input.particle.tau=2.1e-15;              % LSPR lifetime
gamma=1/(2*pi*Input.particle.tau);
A0=0.8*1e-5/(4*pi);                      % scattering amplitude
alpha_static=A0./(2*pi*c./lambda_peak-2*pi*c./lambda-1i*gamma);
```

```
% Long wavelength improvement [See T. Jensen, L. Kelly, A. Lazarides, and G. C. Schatz, ?↙
Electrodynamics
% of noble metal nanoparticles and nanoparticle clusters,? J. Clust. Sci. 10, 295?317↙
(1999)]:
a=180e-9;                       % 100..200e-9 particle dimension (radius of a↙
'sphere'...)
alpha=alpha_static./(1-(2i/3*k.^3).*alpha_static-(k.^2./a).*alpha_static);

%% 3. Construct Result structure containing the data
alpha_star = 1./(1./alpha-S_n_sum);                     % effective polarizability
ext = k.*imag(alpha_star);                              % raw extinction
ext_scaled=ext./(Input.p(1)*Input.p(2)/(4*pi));         % scale extinction by dividing by the↙
atomic number density and 4*pi (from cgs):
T=1-ext_scaled;                                         % transmission

% Make Result structure:
Result.lambda=lambda;
Result.S_n_sum=S_n_sum;
Result.T=T;
Result.alpha_lor=alpha;
Result.alpha_star=alpha_star;
Result.ext=ext;

%% 4. Plot (if needed) the lattice sums and particle polarizabilities
if Input.plotting
    f1=figure(12);
    set(f1,'position',[153    54  1461   846])

    % plot polarizabilities (alpha_lor) and lattice sums (S_n_sum)
    subplot(2,1,1)
    hold on
    plot(lambda*1e9,real(1./alpha))  ;
    plot(lambda*1e9,imag(1./alpha),':');
    Yaxis_lim=[-4*1e21 10*1e21];
    ylim([Yaxis_lim(1) Yaxis_lim(2)])
    xlabel('Wavelength (nm)')
    ylabel('Lattice sum (a.u.)')
    box on

    plot(lambda*1e9,real(S_n_sum),'r-')
    plot(lambda*1e9,imag(S_n_sum),'b:')
    xlim([min(lambda*1e9) max(lambda*1e9)])

    % plot transmission (T)
    subplot(2,1,2)
    hold on
    ax_ext=plot(lambda*1e9,T);
    xlim([min(lambda*1e9) max(lambda*1e9)])
    box on
    xlabel('Wavelength (nm)')
    ylabel('Transmission')
end

end

function [Lattice,S_n_sum_outFP] = Calculate_lattice_sum_FP_sub(Input,k,Tc)
% Calculates the lattice sum, which includes the term due to close-by interface.

n1=Input.n_disp;    % simplify the variable name of the refractive indexs
n2=1;               % assume that the medium above the interface is air

%% 1. Construct the Array position and angle variables X,R and Theta:
r_xi=linspace(0,Input.p(1)*(Input.Njj(1)-1),Input.Njj(1));
```

```
r_xi=r_xi-Input.p(1)*(Input.Njj(1)-1)/2-Input.p(1)/2;       % x-coordinates

r_yi=linspace(0,Input.p(2)*(Input.Njj(end)-1),Input.Njj(end));
r_yi=r_yi-Input.p(2)*(Input.Njj(end)-1)/2-Input.p(2)/2;     % y-coordinates

% build Nx2 r_i as output position vector
[R_i{1},R_i{2}]=meshgrid(r_xi,r_yi);
for ii=1:2 % 3 for 3D
    Array.r_i(:,ii)=single(R_i{ii}(1:end));
end
Arr.R = sqrt(Array.r_i(:,1).^2 + Array.r_i(:,2).^2);

R=Arr.R(Arr.R > 1e-12);          % remove zero R
X=Array.r_i(Arr.R > 1e-12,1);   % remove X with zero R
Theta=acos(X./R);                % angle between x-axis and the direction vector r_i


%% 2. Fabry-Perot interface term here:
% if computer has an GPU, move variables into GPU memory:
if gpuDeviceCount
    Alpha1=gpuArray(atan2(R/2,Tc));
    n1=gpuArray(single(n1));
    R=gpuArray(single(R));
    Tc=gpuArray(single(Tc));
    k=gpuArray(single(k));
else
    Alpha1=atan2(R/2,Tc);       % incidence/reflection angle
end

% 1. calculate angles at which particles can get coupled:
ALPHA1=zeros(length(Alpha1),length(n1),'like',Alpha1);
ALPHA1=repmat(Alpha1,[1 size(n1,1) ]);  % vectorize n1 into N1 [wavelengths, particles]

N1=zeros(length(Alpha1),length(n1),'like',Alpha1);
N1=repmat(n1.',[size(Alpha1,1) 1]);  % vectorize n1 into N1 [wavelengths, particles]

ALPHA2=asin(complex(N1.*sin(ALPHA1)./n2));

% 2. calculate  a) the propagation factor and b) the phase term
OPLtot=zeros(length(R),1,'like',Alpha1);
OPLtot=2.*sqrt((R/2).^2+Tc.^2);

Rp=(N1.*cos(ALPHA1)-n2.*cos(ALPHA2))./(N1.*cos(ALPHA1)+n2.*cos(ALPHA2));
%     Rs=(n2.*cos(ALPHA1)-N1.*cos(ALPHA2))./(n2.*cos(ALPHA1)+N1.*cos(ALPHA2));

% homogeneous environment lattice sum:
SN_array = exp(1i.*R*k.').*((1-1i*R*k.').*...
    (3*cos(Theta).^2-1)./(R.^3) + (k.^2).'.*sin(Theta).^2./R);

% interface addition to the lattice sum:
SN_FP_array =  Rp.*exp(1i.*OPLtot*k.').*((1-1i*(OPLtot)*k.').*...
    (3*cos(Theta).^2-1)./((OPLtot).^3) + (k.^2).'.*sin(Theta).^2./(OPLtot));
% next question is how well this approximates the real Green's function, mjh...

% gather results from the GPU memory (if GPU is used):
if gpuDeviceCount
    S_n_sum_out=gather(sum(SN_array));
    S_n_sum_outFP=gather(sum(SN_FP_array));
else
    S_n_sum_out=sum(SN_array);
    S_n_sum_outFP=sum(SN_FP_array);
end
```

```
%% 3. complile results into Lattice structure:
Lattice.S=squeeze(S_n_sum_out);
Lattice.S_FP=squeeze(S_n_sum_outFP);

end
```
